# Supplementary material for: ReCon: Revealing and Controlling PII Leaks in Mobile Network Traffic
Source: arXiv:1507.00255 source file (2016-08-19)
Supplement: Supplementary file 1 [file appendix.tex]

\appendix
\section{Appendix}

\subsection{Observations from Manual Tests}
\label{app:pinning}
We observed that some iOS apps implemented certificate pinning: Several apps use pinning at least for login and registration (Facebook/Facebook Messenger, WhatsApp, Google, Gmail, Dropbox), others throughout the app's functionality (iTunes U, Vine, Twitter, Periscope). Some games seem to use certificate pinning on startup when they are downloading additional game data (Angry Birds 2, Game of War - Fire Age, Jurassic World). Furthermore, 4 apps prohibited usage over VPN (Snapchat, Snap Upload For Snapchat, OfferUp, Google Translate). Candy Crush Saga produced an error message about not being able to connect to Facebook, yet still had access to the account's friends. Tumblr also seems to perform some kind of certificate checking: It produced an error message about not being able to complete the registration, but the account was still created. Finally, the registration and login for both Netflix and Ibotta did not work with and even without intercepting the traffic.

\subsection{IRB details}
\label{app:irb}
 We are using \recon for an IRB-approved study (\#13-08-04) that reports data from capturing all of a subject's Internet traffic, which raises significant privacy concerns.  
The study protocol entails informed consent from subjects who are interviewed, where the risks and benefits of our study are explained.  
The incentive to use \recon is Amazon.com gift certificates.
To protect the data collected, we use public key cryptography to encrypt the captured data before it is stored on disk. 
Further, subjects can delete their data and disable monitoring at any time. 
Per the terms of our IRB, we cannot make this data public due to privacy concerns.

In our second deployment model, we have IRB approval  (\#13-11-17) for a follow-up study where we record only the first few 
bytes of the HTTP payload, reducing the risk of recording sensitive information. We conduct 
informed consent using an online form, allowing us to enroll users worldwide. The incentive 
to use our system is increased privacy; in return, we collect limited information that allows us 
to validate the effectiveness of \recon and improve its accuracy with user feedback.

\subsection{Full survey results}
\label{app:user-survey}
Table~\ref{table-usurvey} presents the full set of questions and responses from our user study about
the effectiveness of \recon.
 \begin{table}
\centering
\begin{small}

\begin{tabular}{p{180pt}|c}
\textbf{Response} & \textbf{Count} \\ \hline
I spent more time reviewing claims made by applications regarding access to my data, like contacts, location and so on. & 6 \\
I stopped using certain applications because Meddle shows they leak too much personally identifiable information. & 11 \\
I learned to keep location service off unless needed. & 4 \\
I used Meddle to block information that I do not want leaked. & 2 \\
No change. & 3 
\end{tabular}
\end{small}
\caption{ \textbf{User survey results for the question of whether information revealed by \recon changed participant habits.} Most users 
took action to address privacy as a result of information provided by \recon. Some users chose multiple options.}
\label{table-usurvey}
\end{table}

\subsection{Privacy and Incentives}
\label{app:privacy}
Beyond the context of the user study, we will provide incentives and deployment models that balance privacy 
and utility for \recon.  First, we will make our software source code publicly available to build trust 
from users, Second, we will provide easy-to-use hardware and software that allows 
users to run the \recon system on their own devices inside their own network. This substantially 
reduces the privacy risk because user traffic never traverses an untrusted machine, 
and it opens up exciting research opportunities, such as bumping SSL connections 
to identify and block PII in HTTPS flows.  

An interesting challenge is how to incorporate 
a crowdsourced classifier in this deployment model. We believe that we can retrain each 
user's classifier locally based on feedback, then exchange the models themselves with 
other users. Because the models should not contain any PII (rather, they store the features 
associated with PII), the privacy risk should be minimal. However, it is an open question whether 
we can ensure that PII does not leak via side channels.  

\balance

\subsection{Alternative Architectures for PII Sharing}
\label{app:alternative} 
In the current implementation,  \recon relies on being able to identify PII in plaintext flows. Naturally, 
if users begin to block or change their PII using \recon, trackers and advertisers may resort to 
obfuscation and encryption to avoid detection. In response, we can simply retrain \recon to 
identify obfuscated PII leaks, using available static and dynamic analysis tools that are resilient to 
these evasion techniques. Of course, this could lead to an endless cat-and-mouse game of PII detection evasion. 
We hope to avoid this using \recon to promote explicit PII sharing, where users and third 
parties engage in an incentive-driven, mutually beneficial service. In the case that third parties 
choose not to participate in such a scheme, we can provide strong incentives by \emph{blocking all 
traffic to those sites} unless they cooperate.
